# Supplementary material for: Generalized Willmore Energies, Q-Curvatures, Extrinsic Paneitz Operators, and Extrinsic Laplacian Powers
Source: arXiv:2111.00179 ancillary file (2023-03-02)
Supplement: Supplementary file 1 [file FORM-synopsis.pdf]

# FORM DOCUMENTATION FOR *GENERALIZED WILLMORE ENERGIES, $Q$-CURVATURES, EXTRINSIC PANEITZ OPERATORS, AND EXTRINSIC LAPLACIAN POWERS*

SAM BLITZ$^\flat$, A. ROD GOVER$^\sharp$ & ANDREW WALDRON$^\natural$

## 1. Introduction

This note is supplemental material for the paper [2] and documents code used to prove Lemma 7.10, Lemma 7.11, Theorem 7.12, Corollary 1.1, Theorem 4.1, Lemma 5.1, Theorem 5.2, and Theorem 6.2 of [2]. We will also assume basic knowledge of the algebraic manipulation software FORM developed by Jos Vermaseren [4] and funded by FOM, the Dutch granting agency for physics research. A short tutorial can be found in [3] and more detail can be found in the manual [5]. Most of the commands implemented in the attached FORM files are described in [3]. Those commands that are not implemented there will be discussed here.

## 2. New Commands

The primary new structure not found in [3] is a directory containing several *header* and *procedure* files. These are files that do not perform any specific calculations, but instead contain one or more procedures that can be used in essentially any computation. This reduces redundancy and centralizes the more basic identities that are used in many of these FORM computations. All of these files are included in the directory `FORM-Proofs/Headers`. In order to use these files in a given computation, two steps are needed. First, one must include that directory when calling FORM to run; to do so, feed FORM the `-p DIRECTORY-NAME` option at run-time. The second step is to include in the FORM code itself lines that indicate which header (or procedure) files are to be included in that specific program. This is done with a line such as `#include - DIRECTORY/FILENAME.h;`.

Another useful command implemented here is the `delete storage;` command. When called this command removes from memory all globally-stored expressions. By deleting the stored global expressions when we no longer need them in a particular computation, those global expressions can be imported into many different linked computations.

In one instance, we used a special feature of FORM that allows for the counting of the number of arguments a wildcard field may match. Consider the line `id f(?A)= nargs_(?A)`. The keyword `nargs_` takes as input the argument field and returns an integer equaling the number of arguments contained in that argument field. For example, the above line of code would match `f(a,b,c)` to `3`. This particular tool was used in computing the weights of tractor expressions comprised of the action of some number of Thomas-$D$ operators acting on another tractor, where the number of Thomas-$D$ operators was not fixed.

The `renumber` command was also not documented in [3]. This particular command attempts to relabel dummy indices in order to reduce the number of terms. Our implementation `renumber 1;` indicates to FORM that it should try every permutation of dummy indices to try to reduce the number of terms in the output—this typically results in a dramatic simplification of the result.

The `if` command was already discussed in [3]. Here we used that the `if` command can return a boolean `1` or `0` if FORM's pattern-matching machinery would find a match in a term in

2020 *Mathematics Subject Classification.* 53C18, 53A55, 53C21, 58J32.

a given expression. For example, if FORM's active expression was `f(a,b,b)+ f(a,b,c)`, then the line `if(match(f(a?,b?,b?))== 1)id f(a?,b?,c?)= g(a,b,c);` would turn our original expression into `g(a,b,b)+ f(a,b,c)`.

Even though many of the tensors we define in our FORM code have various symmetries, FORM is not particularly adept at handling specific symmetries of tensors, and thus occasionally needs to be prodded to do some simplification via explicit instructions. To that end, the `Symmetrize` and `Antisymmetrize` commands can be useful. While these commands can be implemented in many ways, we used two particular sets of arguments in our computations. Given a declared tensor (with no declared symmetries) `T`, the command `Symmetrize T 1,3;` explicitly symmetrizes the tensor `T` in its first and third indices everywhere that the tensor has at least three indices. Alternatively, the command `Symmetrize T:4 1,2;` will only symmetrize the tensor `T` in the first and second indices when the tensor has exactly four indices—otherwise it does nothing. The `Antisymmetrize` command has the exact same argument types.

## 3. Declarations

In the files `Headers/symbol-index-declarations.h`, `Headers/function-declarations.h`, `Headers/tractor-declarations.h`, and `Headers/Riem-declarations.h`, we declared a number of objects that are associated to particular variables, functions, tractors, and tensors, respectively. For clarity, we provide tables of these declarations and their mathematical counterparts.

First, note that our convention is that (with few exceptions) indices that are enclosed in square brackets `[*]` are to be viewed as "free" or floating indices that are not contracted onto other indices, and the same set of indices without the square brackets are to be viewed as dummy indices. We use lower-case letters at the beginning of the alphabet (except "d") to represent Riemannian indices and upper-case letters at the beginning of the alphabet (except "D") to represent tractor indices. One exception is that we typically use upper-case letters for argument fields, regardless of the type of index that those argument fields represent.

The symbols `d` and `db` represent the dimension of the bulk manifold and the hypersurface respectively. The symbols `x,ep,alpha,beta,invep,invalpha` are dummy variables that typically represent real numbers. In particular, `ep` is often used for dimensional continuation purposes as $\varepsilon$, `invep` is its inverse $\varepsilon^{-1}$, and similarly for `alpha` and `invalpha`.

Some of the scalars and functions not listed in the below table are documented in the FORM file itself. Table 1 contains all of the functions and scalars declared in `Headers/function-declarations.h`. Table 2 contains all of the tractors declared in `Headers/tractor-declarations.h`. Table 3 contains all of the Riemannian tensors declared in `Headers/Riem-declarations.h`.

## 4. Execution

To run the computations, first ensure that FORM is in the path. The version of FORM required to run these computations requires a unix-based operating system, so if one wishes to run these computations on a Windows machine, they must use a linux simulator such as Cygwin and install FORM there. Once FORM is installed in the path, the computations can be easily executed by calling a script using the command `bash FileName.sh`. To clear the saved files, execute the script `DeleteData.sh`. Each script is named according to the result it proves, with the exception of `PreliminaryComputations.sh`, which provides lower-level identities to be used elsewhere.

## References

[1] S. Blitz, A. R. Gover, and A. Waldron. Conformal fundamental forms and the asymptotically Poincaré–Einstein condition. arXiv:2107.10381.

[2] S. Blitz, A. R. Gover, and A. Waldron. Generalized Willmore energies, Q-curvatures, extrinsic Paneitz operators, and extrinsic Laplacian powers. arXiv:2111.00179.

| Function | Mathematical Object |
|---|---|
| `H` | $H$ |
| `Jb` | $\bar{J}$ |
| `r` | $\rho$ |
| `dnr` | $\nabla_n \rho$ |
| `dn2r` | $\nabla_n^2 \rho$ |
| `dn3r` | $\nabla_n^3 \rho$ |
| `J` | $J$ |
| `dnJ` | $\nabla_n J$ |
| `dn2J` | $\nabla_n^2 J$ |
| `RhoNN` | $P_{nn}$ |
| `BachNN` | $B_{nn}$ |
| `sigma` | $\sigma$ |
| `K` | $K$ |
| `Kd` | $\dot{K}$ |
| `Kdd` | $\ddot{K}$ |
| `Kddd` | $\dddot{K}$ |
| `DbDbPdT` | $\hat{\bar{D}}^A \hat{\bar{D}}^B \dot{P}^t_{AB}$ |
| `f` | $f$ |
| `[tau^(5/2-d/2)]` | $\tau^{\frac{5-d}{2}}$ |

| Function | Mathematical Object |
|---|---|
| `h(x)` | $\mathsf{h} + x$ |
| `[1/h](x)` | $\frac{1}{\mathsf{h}+x}$ |
| `[I.D]` | $I \cdot D$ |
| `[I.Dh]` | $I \cdot \hat{D}$ |
| `[Dth.IDh2.Dth]` | $\hat{D}^{T\ A} I \cdot \hat{D}^2 \hat{D}^T_A$ |
| `dn` | $\nabla_n$ |
| `Lap` | $\Delta$ |
| `LapT` | $\Delta^\top$ |
| `LapB` | $\bar{\Delta}$ |
| `R1` | $R_1$ |
| `R2` | $R_2$ |
| `R3` | $R_3$ |
| `R4` | $R_4$ |
| `R` | $\mathcal{R}$ |

TABLE 1. FORM functions and their corresponding mathematical objects.


[3] S. Blitz, A. Rod Gover, and A. Waldron. FORM documentation for *Extrinsic Paneitz operators and Q-curvatures*, included with submission [1].

[4] J. Vermaseren. New features of FORM. arXiv math-ph/0010025, 2000.

[5] J.A.M. Vermaseren, T. Kaneko, J. Kuipers, B. Ruijl, M. Tentyukov, T. Ueda, and J. Vollinga. FORM Reference Manual https://www.nikhef.nl/ form/maindir/documentation/reference/online/online.html (updated 4 October 2018).



♭ CENTER FOR QUANTUM MATHEMATICS AND PHYSICS (QMAP), DEPARTMENT OF PHYSICS, UNIVERSITY OF CALIFORNIA, DAVIS, CA95616, USA

*Email address*: `shblitz@ucdavis.edu`

♯ DEPARTMENT OF MATHEMATICS, THE UNIVERSITY OF AUCKLAND, PRIVATE BAG 92019, AUCKLAND 1142, NEW ZEALAND, AND, MATHEMATICAL SCIENCES INSTITUTE, AUSTRALIAN NATIONAL UNIVERSITY, ACT 0200, AUSTRALIA

*Email address*: `gover@math.auckland.ac.nz`

♮ CENTER FOR QUANTUM MATHEMATICS AND PHYSICS (QMAP), DEPARTMENT OF MATHEMATICS, UNIVERSITY OF CALIFORNIA, DAVIS, CA95616, USA

*Email address*: `wally@math.ucdavis.edu`

| **Tensor** | **Object** |
|---|---|
| D(A) | $D_A$ |
| I(A) | $I_A$ |
| [I](A,B) | $h_{AB} - I_A I_B$ |
| Dhat(A) | $\hat{D}_A$ |
| DhTemp(A) | $\hat{D}_A$ |
| Dth(A) | $\hat{D}^T_A$ |
| DthTemp(A) | $\hat{D}^T_A$ |
| Dthext(A) | $\hat{D}^{T\mathrm{e}}_A$ |
| Db(A) | $\bar{D}_A$ |
| Dbh(A) | $\hat{\bar{D}}_A$ |
| P(A,B) | $P_{AB}$ |
| DK(A,...,C) | $\hat{D}_C \cdots \hat{D}_A K$ |
| DtK(A,...,C) | $\hat{D}^T_C \cdots \hat{D}^T_A K$ |
| DKd(A,...,C) | $\hat{D}_C \cdots \hat{D}_A \dot{K}$ |
| DtKd(A,...,C) | $\hat{D}^T_C \cdots \hat{D}^T_A \dot{K}$ |
| DbKd(A,...,C) | $\hat{\bar{D}}_C \cdots \hat{\bar{D}}_A \dot{K}$ |
| DKdd(A,...,C) | $\hat{D}_C \cdots \hat{D}_A \ddot{K}$ |
| DtP(B,C,A) | $\hat{D}^T_A P_{BC}$ |
| DP(C,D,A,...,B) | $\hat{D}_B \cdots \hat{D}_A P_{CD}$ |
| Pd(A,B) | $\dot{P}_{AB}$ |
| Pdd(A,B) | $\ddot{P}_{AB}$ |
| Pddd(A,B) | $\dddot{P}_{AB}$ |
| DPd(C,D,A,...,B) | $\hat{D}_B \cdots \hat{D}_A \dot{P}_{CD}$ |
| DPdd(C,D,A,...,B) | $\hat{D}_B \cdots \hat{D}_A \ddot{P}_{CD}$ |
| Pdt(A,B) | $\mathring{\top}(\dot{P}_{AB})$ |
| PdT(A,B) | $\dot{P}^t_{AB} := (\bar{r} \circ \mathring{\top})(\dot{P}_{AB})$ |
| DbPdT(A) | $\hat{\bar{D}}^B \dot{P}^t_{AB}$ |
| [Dh, Dh](A,B) | $[\hat{D}_A, \hat{D}_B]$ |
| [Dbh,Dbh](A,B) | $[\hat{\bar{D}}_A, \hat{\bar{D}}_B]$ |

| **Tensor** | **Object** |
|---|---|
| W(A,B,C,D) | $W_{ABCD}$ |
| Wt(A,B,C,D) | $W^{\top}_{ABCD}$ |
| Wb(A,B,C,D) | $\bar{W}_{ABCD}$ |
| Ln(A,B) | $L_{AB}$ |
| DtLn(C,D,A,...,B) | $\hat{D}^T_B \cdots \hat{D}^T_A L_{CD}$ |
| DbLn(C,D,A,...,B) | $\hat{\bar{D}}_B \cdots \hat{\bar{D}}_A L_{CD}$ |
| Fn(A,B) | $F_{AB}$ |
| DbFn(C,D,A,...,B) | $\hat{\bar{D}}_B \cdots \hat{\bar{D}}_A F_{CD}$ |
| Jn(A,B) | $J_{AB}$ |
| DbK(A,...,B) | $\hat{\bar{D}}_B \cdots \hat{\bar{D}}_A K$ |
| Gamma(A,B,C) | $\Gamma_{ABC}$ |
| Wn(A,B,C) | $W_{IABC}$ |
| Wd(A,B,C,D) | $\dot{W}_{ABCD}$ |
| Wdd(A,B,C,D) | $\ddot{W}_{ABCD}$ |
| Wddd(A,B,C,D) | $\dddot{W}_{ABCD}$ |
| DW(A,B,C,D,E,...,F) | $\hat{D}_F \cdots \hat{D}_E W_{ABCD}$ |
| DWd(A,B,C,D,E,...,F) | $\hat{D}_F \cdots \hat{D}_E \dot{W}_{ABCD}$ |
| DWdd(A,B,C,D,E,...,F) | $\hat{D}_F \cdots \hat{D}_E \ddot{W}_{ABCD}$ |
| Wnn(A,B) | $W_{IABI}$ |
| [I,I.Dh](A) | $[I_A, I \cdot \hat{D}]$ |
| [I.Dh,I](A) | $[I \cdot \hat{D}, I_A]$ |
| [hashTr](A,B) | $(h_A\,.\,h_B\,.)^\sharp$ |
| [hashTrB](A,B) | $(\bar{h}_A\,.\,\bar{h}_B\,.)^\sharp$ |
| X(A) | $X_A$ |
| Y(A) | $Y_A$ |
| Z(A,a) | $Z^a_A$ |
| Yb(A) | $\bar{Y}_A$ |
| Zb(A,a) | $\bar{Z}^a_A$ |

TABLE 2. FORM tensors representing tractors and the corresponding tractors (or tractor-valued operators). Note that most of these have corresponding "FORM-commuting" counterparts. The names of these counterparts can be found in the set commTracs.

| Tensor | Object |
|---|---|
| `[G_](a,b)` | $g_{ab}$ |
| `[Gb_](a,b)` | $\bar{g}_{ab}$ |
| `n(a)` | $n_a$ |
| `[d^n^](a,...,b,c)` | $\nabla_a \cdots \nabla_b n_c$ |
| `IInc(a,b)` | $\mathrm{II}_{ab}$ |
| `IIO(a,b)` | $\mathring{\mathrm{II}}_{ab}$ |
| `IIO2(a,b)` | $\mathring{\mathrm{II}}_a^c \mathring{\mathrm{II}}_{cb}$ |
| `IIO3(a,b)` | $\mathring{\mathrm{II}}_a^c \mathring{\mathrm{II}}_c^d \mathring{\mathrm{II}}_{db}$ |
| `dtIIO(a,...,b,c,d)` | $\nabla_a^\top \cdots \nabla_b^\top \mathring{\mathrm{II}}_{cd}$ |
| `dbIIO(a,...,b,c,d)` | $\bar{\nabla}_a \cdots \bar{\nabla}_b \mathring{\mathrm{II}}_{cd}$ |
| `dbivIIO(a)` | $\bar{\nabla} \cdot \mathring{\mathrm{II}}_a$ |
| `FNC(a,b)` | $F_{ab}$ |
| `FO(a,b)` | $\mathring{F}_{ab}$ |
| `dtFO(a,...,b,c,d)` | $\nabla_a^\top \cdots \nabla_b^\top \mathring{F}_{cd}$ |
| `dbFO(a,...,b,c,d)` | $\bar{\nabla}_a \cdots \bar{\nabla}_b \mathring{F}_{cd}$ |
| `dbivFO(a)` | $\bar{\nabla} \cdot \mathring{F}$ |
| `IVO(a,b)` | $\mathring{\mathrm{IV}}_{ab}$ |
| `dbIVO(a,...,b,c,d)` | $\bar{\nabla}_a \cdots \bar{\nabla}_b \mathring{\mathrm{IV}}_{cd}$ |
| `Riemann(a,b,c,d)` | $R_{abcd}$ |
| `RiemannB(a,b,c,d)` | $\bar{R}_{abcd}$ |
| `Weyl(a,b,c,d)` | $W_{abcd}$ |
| `Weyln(a,b,c)` | $W_{abcn}$ |
| `Weylnt(a,b,c)` | $W_{abcn}^\top$ |
| `Weylnn(a,b)` | $W_{nabn}$ |
| `Weylt(a,b,c,d)` | $W_{abcd}^\top$ |
| `dbivWeylnt(a,b)` | $\bar{\nabla}^c W_{a(bc)\hat{n}}^\top$ |
| `Weylb(a,b,c,d)` | $\bar{W}_{abcd}$ |
| `Ric(a,b)` | $Ric_{ab}$ |
| `Rho(a,b)` | $P_{ab}$ |
| `RhoN(a)` | $P_{an}$ |
| `RhoNT(a)` | $P_{an}^\top$ |
| `RhoT(a,b)` | $P_{ab}^\top$ |
| `RhoB(a,b)` | $\bar{P}_{ab}$ |
| `dbRhoB(a,...,b,c,d)` | $\bar{\nabla}_a \cdots \bar{\nabla}_b \bar{P}_{cd}$ |
| `Cotton(a,b,c)` | $C_{abc}$ |
| `CottonT(a,b,c)` | $C_{abc}^\top$ |
| `CottonB(a,b,c)` | $\bar{C}_{abc}$ |
| `CottonN(a,b)` | $C_{nab}$ |

| Tensor | Object |
|---|---|
| `CottonNT(a,b)` | $C_{nab}^\top$ |
| `CottonNTS(a,b)` | $C_{n(ab)}^\top$ |
| `CottonNL(a,b)` | $C_{abn}$ |
| `CottonNLT(a,b)` | $C_{abn}^\top$ |
| `CottonNN(a)` | $C_{ann}$ |
| `delK(a,...,b)` | $\nabla_a \cdots \nabla_b K$ |
| `deltK(a,...,b)` | $\nabla_a^\top \cdots \nabla_b^\top K$ |
| `delbK(a,...,b)` | $\bar{\nabla}_a \cdots \bar{\nabla}_b K$ |
| `deltRhoNN(a,...,b)` | $\nabla_a^\top \cdots \nabla_b^\top P_{nn}$ |
| `delbRhoNN(a,...,b)` | $\bar{\nabla}_a \cdots \bar{\nabla}_b P_{nn}$ |
| `dRho(a,...,b,c,d)` | $\nabla_a \cdots \nabla_b P_{cd}$ |
| `dnRho(a,b)` | $\nabla_n P_{ab}$ |
| `dn2Rho(a,b)` | $\nabla_n^2 P_{ab}$ |
| `dn3Rho(a,b)` | $\nabla_n^3 P_{ab}$ |
| `dnWeylnn(a,b)` | $\nabla_n W_{nabn}$ |
| `dn2Weylnn(a,b)` | $\nabla_n^2 W_{nabn}$ |
| `dbH(a,...,b)` | $\bar{\nabla}_a \cdots \bar{\nabla}_b H$ |
| `Bach(a,b)` | $B_{ab}$ |
| `BachT(a,b)` | $B_{ab}^\top$ |
| `BachB(a,b)` | $\bar{B}_{ab}$ |
| `BachN(a)` | $B_{an}$ |
| `BachNT(a)` | $B_{an}^\top$ |
| `dJ(a,...,b)` | $\nabla_a \cdots \nabla_b J$ |
| `dtJ(a,...,b)` | $\nabla_a^\top \cdots \nabla_b^\top J$ |
| `dbJ(a,...,b)` | $\bar{\nabla}_a \cdots \bar{\nabla}_b \bar{J}$ |
| `dr(a,...,b)` | $\nabla_a \cdots \nabla_b \rho$ |
| `dCotton(a,b,c,d)` | $\nabla_a C_{bcd}$ |
| `dWeyl(a,b,c,d,e)` | $\nabla_a W_{bcde}$ |
| `dBach(a,b,c)` | $\nabla_a B_{bc}$ |
| `[hashR](a,b)` | $(g_a \cdot g_b \cdot)^\sharp$ |
| `[hashRB](a,b)` | $(\bar{g}_a \cdot \bar{g}_b \cdot)^\sharp$ |
| `IIOe(a,b)` | $\mathring{\mathrm{II}}_{ab}^{\mathrm{e}}$ |
| `dnIIOe(a,b)` | $\nabla_n \mathring{\mathrm{II}}_{ab}^{\mathrm{e}}$ |
| `dn2IIOe(a,b)` | $\nabla_n^2 \mathring{\mathrm{II}}_{ab}^{\mathrm{e}}$ |
| `dn3IIOe(a,b)` | $\nabla_n^3 \mathring{\mathrm{II}}_{ab}^{\mathrm{e}}$ |
| `dbf(a,...,b)` | $\bar{\nabla}_a \cdots \bar{\nabla}_b f$ |
| `grdivIIoS(a,b)` | $\bar{\nabla}_{(a} \bar{\nabla} \cdot \mathring{\mathrm{II}}_{b)}$ |
| `grdivIIoA(a,b)` | $\bar{\nabla}_{[a} \bar{\nabla} \cdot \mathring{\mathrm{II}}_{b]}$ |

Table 3. FORM tensors representing Riemmanian tensors and the corresponding tensors (or tensor-valued operators). Note that most of these have corresponding FORM-commuting counterparts. The names of these counterparts can be found in the set `commTens`.
